# Supplementary material for: Testing for directed information graphs
Source: arXiv:2108.11074 source file (2021-08-25)
Supplement: Supplementary file 1 [file Appendix_C.tex]

We first begin with expanding $I^{(k)}_n (\co{\bb{X}\to\bb{Y}}{\bb{Z}})$ as below:
\begin{align}
& I^{(k)}_n (\co{\bb{X}\to\bb{Y}}{\bb{Z}})\nonumber\\
&=\sum_{x_1^{k+1} y_1^{k+1} z_1^{k+1}}\hat P(x_1^{k+1} y_1^{k+1} z_1^{k+1}) \log\frac{\hat P(y_k x_1^{k+1}|y_1^k z_1^{k+1})}{\hat P(y_k|y_1^k z_1^{k+1})\hat P(x_1^{k+1}|y_1^k z_1^{k+1})}\nonumber\\
&=\sum_{x_1^{k+1} y_1^{k+1} z_1^{k+1}}\hat P(x_1^{k+1} y_1^{k+1} z_1^{k+1}) \nonumber\\
&\qquad\times\log\biggl[\frac{\hat P(y_k x_1^{k+1}|y_1^k z_1^{k+1})\bar P(y_k|y_1^k z_1^{k+1})\bar P(x_1^{k+1}|y_1^k z_1^{k+1})}{\hat P(y_k|y_1^k z_1^{k+1})\hat P(x_1^{k+1}|y_1^k z_1^{k+1})\bar P(y_k x_1^{k+1}|y_1^k z_1^{k+1})}\nonumber\\
&\quad+\sum_{x_1^{k+1} y_1^{k+1} z_1^{k+1}}\hat P(x_1^{k+1} y_1^{k+1} z_1^{k+1}) \log\frac{\bar P(y_k x_1^{k+1}|y_1^k z_1^{k+1})}{\bar P(y_k|y_1^k z_1^{k+1})\bar P(x_1^{k+1}|y_1^k z_1^{k+1})}\nonumber\\
&=\sum_{x_1^{k+1} y_1^{k+1} z_1^{k+1}}\hat P(x_1^{k+1} y_1^{k+1} z_1^{k+1}) \nonumber\\
&\qquad \times\log\frac{\hat P(x_1^{k+1} y_0^{k} z_1^{k+1}) \hat P(y_1^k z_1^{k+1})}{\hat P(y_0^{k} z_1^{k+1})\hat P(x_1^{k+1} y_1^k z_1^{k+1})} \frac{\bar P(y_0^{k} z_1^{k+1})\bar P(x_1^{k+1} y_1^k z_1^{k+1})}{\bar P(x_1^{k+1} y_0^{k} z_1^{k+1}) \bar P(y_1^k z_1^{k+1})}\nonumber\\
&\quad+\sum_{x_1^{k+1} y_1^{k+1} z_1^{k+1}}\hat P(x_1^{k+1} y_1^{k+1} z_1^{k+1}) \log\frac{\bar P(y_k x_1^{k+1}|y_1^k z_1^{k+1})}{\bar P(y_k|y_1^k z_1^{k+1})\bar P(x_1^{k+1}|y_1^k z_1^{k+1})}\nonumber\\
&=D(\co{\hat P_{X_1^{k+1} Y_1^{k+1} Z_1^{k+1}}}{\bar P_{X_1^{k+1} Y_1^{k+1} Z_1^{k+1}}}) + 
D(\co{\hat P_{Y_1^k Z_1^{k+1}}}{\bar P_{Y_1^k Z_1^{k+1}}})\nonumber\\
&\quad-D(\co{\hat P_{Y_0^{k} Z_1^{k+1}}}{\bar P_{Y_0^{k} Z_1^{k+1}}})-D(\co{\hat P_{X_1^{k+1} Y_1^k Z_1^{k+1}}}{\bar P_{X_1^{k+1} Y_1^k Z_1^{k+1}}})\nonumber\\ 
&\quad+ \sum_{x_1^{k+1} y_1^{k+1} z_1^{k+1}}\left(\frac{1}{n-k}\sum_{i=k}^{n-1}\mathds{1}[X_{i-k}^{i} Y_{i-k}^{i} Z_{i-k}^{i}=x_1^{k+1} y_1^{k+1} z_1^{k+1}]\right)\nonumber\\
&\hspace{2cm}\times\log\frac{\bar P(y_k x_1^{k+1}|y_1^k z_1^{k+1})}{\bar P(y_k|y_1^k z_1^{k+1})\bar P(x_1^{k+1}|y_1^k z_1^{k+1})}.\label{DI_expansion}
\end{align}
As $n\to \infty$ KL-divergence terms in (\ref{DI_expansion}) decay faster than $\mathcal{O}(\frac{1}{\sqrt{n}})$ which we will show later. Then we conclude that,
\begin{align}
&\lim_{n\to\infty} \sqrt{n-k} I^{(k)}_n (\co{\bb{X}\to\bb{Y}}{\bb{Z}})=\frac{1}{\sqrt{n-k}}\sum_{i=k}^{n-1}S_i
\end{align}
where
\begin{align}
S_i\triangleq\log\frac{ P_{\bar Y_k \bar X_1^{k+1}|\bar Y_1^k \bar Z_1^{k+1}}(Y_i X_{i-k}^i|Y_{i-1}^{i-k-1} Z_{i-k}^i)}{P_{\bar Y_k|\bar Y_1^k \bar Z_1^{k+1}}(Y_i|Y_{i-1}^{i-k-1} Z_{i-k}^i)}\nonumber\\
-\log P_{\bar X_1^{k+1}|\bar Y_1^k \bar Z_1^{k+1}}(X_{i-k}^i|Y_{i-1}^{i-k-1} Z_{i-k}^i).\nonumber
\end{align}
Noting that $\mathds{E}[S]=I(\bar Y_k;\bar X_{0}^{k}|\bar Y_{0}^{k-1},\bar Z_{0}^{k})$ and using standard Lindeberg-L\'{e}vy central limit theorem, 
\begin{align}
\sqrt{n-k}\left(\frac{1}{n-k}\sum_{i=k}^{n-1}S_i - \mathds{E}[S]\right)\to \mathcal{N}(0,\sigma^2)
\end{align}
where $\sigma^2$ is bounded. Now to complete the proof, it only remains to show KL-divergence terms in (\ref{DI_expansion}) multiplied with $\sqrt{n-k}$ factor converge to zero as $n\to\infty$. We present the proof for one term and the rest would follow similar approach. We begin with recalling Taylor expansion with Lagrange remainder form, 
\begin{align}
&f(x)=f(a)+f'(a)(x-a)\nonumber\\
&\hspace{1cm}+\frac{f''(x^*) (x-x^*)(x-a)}{2!} \quad x^*\in (a,x).
\end{align}
Define $\rho\triangleq \frac{\bar P(x_1^{k+1} y_1^{k+1} z_1^{k+1})}{\hat P(x_1^{k+1} y_1^{k+1} z_1^{k+1})},$ then we can now expand KL-divergence as:
\begin{align}
&\sqrt{n-k}\, D(\co{\hat P_{X_1^{k+1} Y_1^{k+1} Z_1^{k+1}}}{\bar P_{X_1^{k+1} Y_1^{k+1} Z_1^{k+1}}})\nonumber\\
&= -\sqrt{n-k}\sum_{x_1^{k+1} y_1^{k+1} z_1^{k+1}}\hat P(x_1^{k+1} y_1^{k+1} z_1^{k+1})\log\rho\\
&= -\sqrt{n-k}\sum_{x_1^{k+1} y_1^{k+1} z_1^{k+1}}\hat P(x_1^{k+1} y_1^{k+1} z_1^{k+1})[(\rho-1) - \frac{(\rho-1)(\rho-\tau)}{2!\tau^2}]\\
&= \sqrt{n-k}\sum_{x_1^{k+1} y_1^{k+1} z_1^{k+1}}\hat P(x_1^{k+1} y_1^{k+1} z_1^{k+1})(\rho-1)(\rho-\tau)\frac{1}{2\tau^2}\\
&= \sqrt{n-k}\sum_{x_1^{k+1} y_1^{k+1} z_1^{k+1}}\left(\hat P(x_1^{k+1} y_1^{k+1} z_1^{k+1})-\bar P(x_1^{k+1} y_1^{k+1} z_1^{k+1})\right)^2C
\end{align}
for some $\tau\in (\rho,1 )$ where $$C\triangleq\frac{(\rho -\tau)}{2(\rho -1)\hat P(x_1^{k+1} y_1^{k+1} z_1^{k+1})\tau^2}.$$
Since the Markov model was assumed to be ergodic, $\hat P(x_1^{k+1} y_1^{k+1} z_1^{k+1})\nrightarrow 0$, so $C$ is bounded. 
Now consider sequence of $$Y_i(x_1^{k+1} x_1^{k+1} x_1^{k+1})\triangleq\mathds{1}[X_i^{k+i} Y_i^{k+i} Z_i^{k+i}=x_1^{k+1} x_1^{k+1} x_1^{k+1}],\,\forall i\in[1,n-k]$$ with mean $\bar P(x_1^{k+1} y_1^{k+1} z_1^{k+1})$.
As a result,
\begin{align}
&\sqrt{n-k}\, D(\co{\hat P_{X_1^{k+1} Y_1^{k+1} Z_1^{k+1}}}{\bar P_{X_1^{k+1} Y_1^{k+1} Z_1^{k+1}}})=\frac{\log\log (n-k)}{\sqrt{n-k}}\nonumber\\
&\qquad\times\sum_{x_1^{k+1} y_1^{k+1} z_1^{k+1}}{\left(\hat P(x_1^{k+1} y_1^{k+1} z_1^{k+1})-\bar P(x_1^{k+1} y_1^{k+1} z_1^{k+1})\right)^2}\frac{C(n-k)}{\log\log (n-k)}\label{expansion_D_seq}
\end{align}
According to law of iterated logarithms, $$\lim_{n\to\infty}\frac{\sum_{i=1}^{n-k}(Y_i - \bar P(x_1^{k+1} y_1^{k+1} z_1^{k+1}))}{\sqrt{(n-k)\log\log(n-k)}}=\sqrt{2}.$$
Now by definition of empirical distribution,
$$\lim_{n\to\infty}\frac{\sqrt{(n-k)}(\hat P(x_1^{k+1} y_1^{k+1} z_1^{k+1})-\bar P(x_1^{k+1} y_1^{k+1} z_1^{k+1}))}{\sqrt{\log\log(n-k)}}=\sqrt{2}.$$
Combining this with (\ref{expansion_D_seq}), we conclude that
$$\lim_{n\to\infty}\sqrt{n-k}\, D(\co{\hat P_{X_1^{k+1} Y_1^{k+1} Z_1^{k+1}}}{\bar P_{X_1^{k+1} Y_1^{k+1} Z_1^{k+1}}})=0,$$
and the proof is completed.
\hfil{\qed}
