# Supplementary material for: Testing for directed information graphs
Source: arXiv:2108.11074 source file (2021-08-25)
Supplement: Supplementary file 2 [file Appendix_B.tex]

The proof is analogous to proof of Proposition.9 in \cite{kontoyiannis2016estimating}. Using the definition of log-likelihood,
\begin{align}
& L^{\theta^{\star}}_n(X_1^n,Y_1^n,Z_1^n)\nonumber\\
&=\max\limits_{\theta\in\Theta}\sum_{i=k+1}^{n} \log(Q_{\theta}(X_i,Y_i,Z_i|X_{i-k}^{i-1},Y_{i-k}^{i-1},Z_{i-k}^{i-1}))\nonumber\\
& =\max\limits_{\theta\in\Theta}\sum_{x_1^{k+1}y_1^{k+1}z_1^{k+1}} (n-k)\hat P_{X_1^{k+1}Y_1^{k+1}Z_1^{k+1}}(x_1^{k+1}y_1^{k+1}z_1^{k+1})\nonumber\\
&\qquad\times\log(Q_{\theta}(x_{k+1}y_{k+1}z_{k+1}|x_1^{k}y_1^{k}z_1^{k}))\nonumber\\
&=-(n-k)\biggl[\min\limits_{\theta\in\Theta}\biggl\{D\left(\co{\hat P_{X_1^{k+1}Y_1^{k+1}Z_1^{k+1}}}{Q_{\theta}\otimes \hat P_{X_1^kY_1^kZ_1^k}}\right)\biggr\}\nonumber\\
&+\sum_{x_1^{k+1}y_1^{k+1}z_1^{k+1}}\hat P(x_1^{k+1}y_1^{k+1}z_1^{k+1})\log(\frac{\hat P(x_1^{k}y_1^{k}z_1^{k})}{\hat P(x_1^{k+1}y_1^{k+1}z_1^{k+1})})\biggl]\label{loglikelihood_expansion}
\end{align}
 where 
\begin{align}
&(Q_{\theta}\otimes \hat P_{X_1^kY_1^kZ_1^k})(x_1^{k+1}y_1^{k+1}z_1^{k+1})\triangleq\nonumber\\
&\qquad \hat P_{X_1^kY_1^kZ_1^k}(x_1^{k}y_1^{k}z_1^{k})Q_{\theta}(x_{k+1}y_{k+1}z_{k+1}|x_1^{k}y_1^{k}z_1^{k}).\nonumber
\end{align}
 Since KL-divergence is minimized to zero, then
\begin{align}
& L^{\theta^{\star}}_n(X_1^n,Y_1^n,Z_1^n)\nonumber\\
&\qquad =(n-k)[\hat H(X_1^k,Y_1^k,Z_1^k)-H(X_1^{k+1},Y_1^{k+1},Z_1^{k+1})]\label{likelihood1}
\end{align}
On the other hand, for the second log-likelihood, we have:
\begin{align}
& L^{\phi^{\star}}_n(X_1^n,Y_1^n,Z_1^n)\nonumber\\
&=\max\limits_{\phi\in\Phi}\sum_{i=k+1}^{n} \log(Q_{\phi}(X_i,Y_i,Z_i|X_{i-k}^{i-1},Y_{i-k}^{i-1},Z_{i-k}^{i-1}))\nonumber\\
&=\underbrace{\max\limits_{\phi^{xz}}\sum_{i=k+1}^{n} \log(Q_{\phi^{xz}}(X_i,Z_i|X_{i-k}^{i-1},Y_{i-k}^{i-1},Z_{i-k}^{i-1}))}_{T_1}
\nonumber\\
&\quad+\underbrace{\max\limits_{\phi^{y}}\sum_{i=k+1}^{n}\log(Q_{\phi^y}(Y_i|Y_{i-k}^{i-1},Z_{i-k}^{i}))}_{T_2}.\nonumber
\end{align}
With similar approach as \eqref{loglikelihood_expansion} we can expand $T_1$ and $T_2$ as follows:
\begin{align}
& T_1=\nonumber\\
&\, -(n-k)\biggl[\min\limits_{\phi^{xz}}\bigl\{D(\co{\hat P_{X_1^{k+1},Y_1^{k},Z_1^{k+1}}}{Q_{\phi^{xz}}\otimes \hat P_{X_1^{k},Y_1^{k},Z_1^{k}}})\bigr\}\nonumber\\
&\, +\sum_{x_1^{k+1},y_1^{k},z_1^{k+1}}\hat P(x_1^{k+1},y_1^{k},z_1^{k+1})\log(\frac{\hat P(x_1^{k},y_1^{k},z_1^{k})}{\hat P(x_1^{k+1},y_1^{k},z_1^{k+1})})\biggr]\\
& T_2=\nonumber\\
&\, -(n-k)\biggl[\min\limits_{\phi^{y}}\bigl\{D(\co{\hat P_{Y_1^{k+1},Z_1^{k+1}}}{Q_{\phi^{y}}\otimes\hat P_{Y_1^{k},Z_1^{k+1}}})\bigr\}\nonumber\\
&\, +\sum_{y_1^{k+1},z_1^{k+1}} \hat P(y_1^{k+1},z_1^{k+1})\log(\frac{\hat P(y_1^{k},z_1^{k+1})}{\hat P(y_1^{k+1},z_1^{k+1})})\biggr].
\end{align}

As a result,
\begin{align}
& L^{\phi^{\star}}_n(X_1^n,Y_1^n,Z_1^n)=(n-k)\biggl[\hat H(X_1^{k},Y_1^{k},Z_1^{k})\nonumber\\
&-\hat H(X_1^{k+1},Y_1^{k},Z_1^{k+1}) + \hat H(Y_1^{k},Z_1^{k+1})-\hat H(Y_1^{k+1},Z_1^{k+1}) \biggr]\label{likelihood2}
\end{align}
Combining \eqref{likelihood1} and \eqref{likelihood2} we obtain
\begin{align}
&\Lambda_{{xy},n}= L^{\theta^{\star}}_n(X_1^n,Y_1^n,Z_1^n)-L^{\phi^{\star}_{xy}}_n(X_1^n,Y_1^n,Z_1^n)\nonumber\\
&=(n-k)[\hat H(X_1^{k+1},Y_1^{k},Z_1^{k+1})-\hat H(X_1^{k+1},Y_1^{k+1},Z_1^{k+1})\nonumber\\
&\hspace{3.55cm}- \hat H(Y_1^{k},Z_1^{k+1})+\hat H(Y_1^{k+1},Z_1^{k+1})]\nonumber\\
&=(n-k)[\hat H(Y_{k+1}|Y_1^k,Z_1^{k+1})-\hat H(Y_{k+1}|X_1^{k+1},Y_1^{k},Z_1^{k+1})]\nonumber\\
&=(n-k)\hat I_n^{(k)}(\co{\bb{X}\to\bb{Y}}{\bb{Z}})
\end{align}
\hfil{\qed}
